# Supplementary material for: Configurational microcanonical statistical mechanics from Riemannian geometry of equipotenital level sets
Source: arXiv:2205.14536 source file (2022-05-28)
Supplement: Supplementary file 1 [file appendix1.tex]

\section{System initialization}

\subsection{$\text{C}_{70}$-phenyl ring structure: Details and analysis}

\subsubsection{Reprojection of MBD energy among fragments to effective PW interaction energy}
\begin{itemize}
    \item MBD interaction energy $E_{\rm MBD}$  contains all the the N-body contributions of interaction energy among fragments. Let us consider a system $\mathcal{S}=\bigcup_{k=1}^{N} \mathcal{F}_K$ made of $N$ fragments.\\
    The MBD energy $\epsilon_{i_1,...,i_K}$ of K fragments with $i_1<....<i_K$ is given by 
    \begin{equation}
        \epsilon_{i_1,...,i_k}=\langle \Psi_{\mathrm{MBD},i_1,...,i_K} |\sum_{j=i_1}^{i_K}\left[\hat{H}_{0i_j}+\sum_{i_l<i_j}\hat{V}_{i_l,i_j}\right]| \Psi_{\mathrm{MBD},i_1,...,i_K}\rangle-\langle \Psi_{0,i_1,...,i_K} |\sum_{j=i_1}^{i_K}\hat{H}_{0i_j}| \Psi_{0,i_1,...,i_K}\rangle
    \end{equation}

    i.e. \cite{kaplan2006intermolecular}
    \begin{equation}
       E_{\rm MBD}(\mathcal{S})=E_{1\mathrm{B}}(\mathcal{S})+E_{2\mathrm{B}}(\mathcal{S})+....+E_{N\mathrm{B}}(\mathcal{S})
    \end{equation}
    where
    
    \end{itemize}
\subsubsection{Many Body decomposition analysis of $\rm{C}_{70}@\rm{CPPA}[8]$ configuration of Fig.1}
\begin{figure}[h!]
\centering
\includegraphics[scale=0.4]{Figures/AppendixA/C70-in-8CPPA_along_distmatr_CGI_lmbd.png}
\caption{Distance matrix for the first level of coarse graining of the $\text{C}_{70}@[8]\text{CPPA}$ configuration reported in Fig.1 }
    \label{fig:my_label}
\end{figure}
\begin{figure}[h!]
    \centering
    \includegraphics[scale=0.4]{Figures/AppendixA/covergenceMBDexpansion.pdf}
    \caption{Convergence of many body expansion of the total dispersion energy of the system $E_{\rm{kBD}}(\mathcal{S})$ and the potential energy $V_{\rm{kBD}}(\mathcal{S})$ for the set of fragments $\mathcal{S}=\{\text{C}_{70},\text{CPPA}_1,...,\text{CPPA}_8\}$ for the geometry considered in Fig.1}
    \label{fig:my_label}
\end{figure}

\begin{figure}
    \centering
    \includegraphics[scale=0.55]{Figures/AppendixA/C70-in-8CPPA_along_imgprjDeltaU1FvsETS_CGI_lmbd.png}
    \caption{Difference between the MBD energy and internal TS for each fragment in the geometry of Fig.1 . The difference in the total energy of the $\text{C}_{70}$ fullerene sphere has not been reported as 
    its value is out of scale as $U_{1\rm{F}D}(\text{C}_{70})-U_{\rm{TS}}(\text{C}_{70}) \approx -\SI{229.3}{\milli\electronvolt}$.}
    \label{fig:my_label}
\end{figure}

\begin{figure}[h!]
\begin{minipage}{0.32\textwidth} \includegraphics[scale=0.33]{Figures/AppendixA/C70-in-8CPPA_along_eint2mbdVseintTS_CGI.png}
\end{minipage}
\hfill
\begin{minipage}{0.32\textwidth}
    \includegraphics[scale=0.33]{Figures/AppendixA/C70-in-8CPPA_along_eint3mbdVseint2mbd_CGI.png}
\end{minipage}
\hfill
\begin{minipage}{0.32\textwidth}
    \includegraphics[scale=0.33]{Figures/AppendixA/C70-in-8CPPA_along_eint4mbdVseint3mbd_CGI.png}
\end{minipage}
\centering
    \caption{Correction at any successive order of k-body dispersion on PW interactions}
    \label{fig:my_label}
\end{figure}

\begin{figure}[h!]
\begin{minipage}{0.4\textwidth}
     \centering
        \includegraphics[scale=0.35]{Figures/AppendixA/C70-in-8CPPA_along_corre4FDvsdist_lmbd_CGI.png}   
\end{minipage}
\hfill
\begin{minipage}{0.4\textwidth}
     \centering
        \includegraphics[scale=0.5]{Figures/AppendixA/C70-in-8CPPA_along_effk_lmbd_CGI.png}   
\end{minipage}
\caption{Estimation of the spatial range of 4FD interactions
re-projected between pair of fragments.}
    \label{fig:my_label}
\end{figure}

\clearpage
\newpage

\subsubsection{Many-fragment dispersion energy for varying geometries}

\begin{figure}[h!]
\begin{minipage}{0.4\textwidth}
     \centering
        \includegraphics[scale=0.35]{Figures/Figure3/center/interdekImg4FD.png}   
\end{minipage}
\hfill
\begin{minipage}{0.4\textwidth}
     \centering
        \includegraphics[scale=0.35]{Figures/Figure3/center/interdekImg.png}   
\end{minipage}
\caption{Interpolation of $\Delta k_{4\text{FD}/TS}$ and $\Delta k_{\rm{prjMBD}/TS}$ for the symmetric $\text{C}_{70}$@[8]CPPA geometry of Fig.3}
    \label{fig:my_label}
\end{figure}

\begin{figure}[h!]
\begin{minipage}{0.4\textwidth}
     \centering
        \includegraphics[scale=0.35]{Figures/Figure3/side/interdekImg4FD.png}   
\end{minipage}
\hfill
\begin{minipage}{0.4\textwidth}
     \centering
        \includegraphics[scale=0.35]{Figures/Figure3/side/interdekImg.png}   
\end{minipage}
\caption{Interpolation of $\Delta k_{4\text{FD}/TS}$ and $\Delta k_{\rm{prjMBD}/TS}$ for the asymmetric $\text{C}_{70}$@[8]CPPA geometry of Fig.3}
    \label{fig:my_label}
\end{figure}

\clearpage
\newpage
\subsection{Crambin}
\subsubsection{Coarse-graining by residues}

\begin{figure}[h!]
\begin{minipage}{0.4\textwidth}
     \centering
        \includegraphics[scale=0.5]{Figures/Protein/residue/distmatrfrag.png}
        \end{minipage}
\caption{Distance Matrix for the mutual distance among the residues centers of mass}
    \label{fig:my_label}
\end{figure}

\begin{figure}[h!]
\begin{minipage}{0.4\textwidth}
     \centering
        \includegraphics[scale=0.35]{Figures/Protein/residue/ImgcorrdistVMBDff.png}   
\end{minipage}
\hfill
\begin{minipage}{0.4\textwidth}
     \centering
        \includegraphics[scale=0.35]{Figures/Protein/residue/Imgcorrdist4FDV.png}
\end{minipage}
\caption{Correlation between the }
    \label{fig:my_label}
\end{figure}

\begin{figure}[h!]
\begin{minipage}{0.4\textwidth}
     \centering
        \includegraphics[scale=0.35]{Figures/Protein/residue/ImgcorrdistPWMBDonTS.png}   
\end{minipage}
\caption{Correlation between the  }
    \label{fig:my_label}
\end{figure}

\subsubsection{Coarse-graining by secondary structures}

\subsection{DNA models}
DFTB calculations to determine the mean field electronic ground state performed with
