# Supplementary material for: Configurational microcanonical statistical mechanics from Riemannian geometry of equipotenital level sets
Source: arXiv:2205.14536 source file (2022-05-28)
Supplement: Supplementary file 2 [file appendix2.tex]

\section{The QDOs/MBD model}
The correlation energy in an electronic system
can be calculated from the semi-classical ACFD formula,
\begin{equation}
\label{eq:ACFD_original}
    E_{\text{corr}}=-\dfrac{1}{2\pi}\int\limits_{0}^{+\infty}\mathrm{d}\omega\int_{0}^{1}\mathrm{d}\lambda\int\int \mathrm{d}\mathbf{r}\mathrm{d}\mathbf{r}'\left[\chi_{\lambda}(\mathbf{r},\mathbf{r}',\mathrm{i}\omega)-\chi_{\lambda=0}(\mathbf{r},\mathbf{r}',\mathrm{i}\omega)\right]\mathcal{V}_{\text{coul}}(\mathbf{r},\mathbf{r}')
\end{equation}
where $\mathcal{V}_{\text{coul}}(\mathbf{r},\mathbf{r}')=\|\mathbf{r}-\mathbf{r}'\|$ is the Coulomb potential and $\chi_{\lambda}(\mathbf{r},\mathbf{r}',\omega)$ is Fourier transform in frequency domain of the density-density response function of the electronic density at point $\mathbf{r}$ and time t to a perturbation at the position $\mathbf{r}'$ at a frequency $\omega$ (the immaginary part describing the contribution due to dissipation).\\
In a system composed of $N$ fragments (i.e. atoms) in presence of a finite electronic
gap in spectrum a coarse-grained simplified version of Eq.\eqref{eq:ACFD_original} in random phase approximation (i.e. ignoring 
the correlations due to exchange interactions).[...]
% derived in systems with a finite electronic gap,introducing the non-local frequency-dependent polarizability tensor $\boldsymbol{\alpha}(\mathbf{r},\mathbf{r}',\mathrm{i}\omega)$The random phase approximation (ignoring the exchange-correlations)
Dispersive many-body interactions in a system of N atoms can be effectively described by a system of three dimensional Quantum Drude Oscillators (QDOs)
coupled through coulombic interactions in dipole-dipole
approximation representing quantum electronic fluctuation around each atom.
The Hamiltonian of the QDOs/MBD model reads,
\begin{equation}
    \hat{H}(\hat{\mathbf{p}},\hat{\mathbf{x}})=\sum\limits_{A=1}^{N}\left[ \dfrac{\|\hat{\mathbf{p}}_A\|^2}{2}+\dfrac{1}{2}\hat{\mathbf{x}}_{A} \mathcal{T}_{AB}(\mathbf{R}_A,\mathbf{R}_B) \hat{\mathbf{x}}_{B}\right]
\end{equation}
where $\hat{x}_{A,i}=\sqrt{m_{A}}(\hat{r}_{A,i}-R_{A,i})$ is the $i$-th cartesian component of the (mass scaled) displacement of the Drude particle with respect to the position of the atomic center $\mathbf{R}_{A}$. 
The potential energy matrix
\begin{equation}
\mathcal{T}_{AB,ij}(\mathbf{R}_A,\mathbf{R}_B)=\omega_{A}\omega_{B}\left[\delta_{AB}\delta_{ij}+\dfrac{q_Aq_B}{\omega_{A}\omega_{B}m_A^{\frac{1}{2}}m_B^{\frac{1}{2}}}\nabla_{\mathbf{R}_{A,i}}\otimes \nabla_{\mathbf{R}_{B,i}} \mathcal{V}_{\text{ESpot}}(\mathbf{R}_{A},\mathbf{R}_{B})\right]
\end{equation}
is a $3 \times 3$ real matrix where $\omega_A$, $m_A$ and $q_A$ are respectively the angular frequency, the effective mass and the effective charge\footnote{Gaussian units are used, i.e. the electric charge has dimensions  $[q]=([\text{Energy}][\text{length}])^{\frac{1}{2}}=([\text{mass}][\text{length}]^{3}[\text{time}]^2)^{\frac{1}{2}}$ while the polarizability has dimensions of a volume $[\alpha]=[\text{length}]^3$ } of the $A$-th Drude oscillator and
$\mathcal{V}_{\text{ESpot}}$ is the electrostatic potential among charges.\\
If $\mathcal{V}_{\text{ESpot}}=\mathcal{V}_{\text{coul}}$, so assuming the electrostatic interaction potential among point-like charge distributions, this leads to the so called "polarizability catartophe", i.e. the total interaction matrix
$$\mathrm{T}_{\alpha\beta}=\mathcal{T}_{AB,ij}\delta_{3(A-1)+i,\alpha} \delta_{3(B-1)+j,\alpha}$$ is not positive definite.
In the self-consistent screening (SCS) method, introduced to calculate the rescaling
of atomic polarizability due to dipole-dipole interactions
among QDOs at short distances, it has been proposed to adopt for $\mathcal{V}_{\text{ESpot}}$ the electrostatic potential among two isotropic gaussian distribution of equal charge
\begin{equation}
    \mathcal{V}_{\text{Gpot}}(\mathbf{R}_A,\mathbf{R}_B)=\dfrac{\text{erf}\left[\|\mathbf{R}_B-\mathbf{R}_A\|/\sigma_A\right]}{\|\mathbf{R}_B-\mathbf{R}_A\|}
\end{equation}
where $\sigma_{AB}=\sqrt{\sigma_A^2+\sigma_B^2}$ being $\sigma_A$ the width of the gaussian single charge distribution, i.e. $$\rho(\mathbf{r})=\|\psi(\mathbf{r})\|^2=\dfrac{\exp\left[-\|\mathbf{r}-\mathbf{R}\|^2 /(2\sigma)\right]}{\pi^{\frac{3}{2}}\sigma^3}$$.\\

Fixing the parameter $\{m_{A},\omega_A,q_A\}$ for each harmonic oscillator of each  atomic QDOs is a crucial aspect of the QDOs/MBD model. For an atom in free space it is possible to parametrize Drude oscillator in terms of the static polarizability $\alpha_{A,\text{free}}$ and the $C_{6AA}$-interaction coefficient
parametrizing the pairwise van der Waals
among identical atoms.
The static polarizability QDO representing the electronic response of the $A$-th in its ground state is given by
\begin{equation}
\label{eq:alpha_cond}
    \alpha_{A}(0)=\dfrac{q_A^2}{m_A\omega_A^2}\,\,\,.
\end{equation}
A second condition to parametrize the Drude Oscillator can be derived in terms of the 
$C_{6AA}$ describing pairwise vDW interactions among identical atoms using Casimir-Polder integral
\begin{equation}
\label{eq:C6_CasPol}
C_{6AA}=\dfrac{3}{\pi}\int_{0}^{\infty} \left[\alpha_{A}(\mathrm{i}\omega)\right]^2 \,\,\mathrm{d}\omega
\end{equation}
and assuming the dynamical atomic polarizability is well approximated by the QDO one,
i.e.
\begin{equation}
    \alpha_{A,\text{QDO}}(\mathrm{i}\omega)=\dfrac{\alpha_{A}(0)}{1+\left(\omega/\omega_{A}\right)^2}\,\,
\end{equation}
and substituting this expression in Eq.\eqref{eq:C6_CasPol} the $C_{6AA,\text{QDO}}$ coefficient reads
\begin{equation}
\label{eq:C6_cond}
 C_{6AA}=\dfrac{3}{4}\hbar\omega_{A}\alpha_{A}^2(0)=\dfrac{3 \hbar q_{A}^4}{4 m_{A}^2 \omega_{A}^3}\,.
\end{equation}
A third independent condition to fix the parameter for Drude oscillator is derived using the characteristic width of an isotropic 3D gaussian distribution.
The probability distribution of a Drude particle in its ground state is given by 
$\rho_{\text{QDO}}(\mathbf{r})=\|\psi_{A}(\mathbf{r})\|^2=\sqrt{m_A\omega_A/(\pi \hbar)}\exp[-\|\mathbf{r}\|^2/(2\sigma_{A}^2)]$ where $\sigma_{A}=\sqrt{\hbar/(2m_A\omega_{A})}$ is the characteristic
width of an harmonic oscillator. 
Moreover, the width of a QDO in its ground state is directly related to the polarizability
in classical electrodynamics and can be derived from the dipole self-energy \cite{mayer2007formulation} so that $\sigma_{A}=(\sqrt{2/\pi}\,\,\alpha_{A}(0)/3)^{\frac{1}{3}}$
from which it follows
\begin{equation}
\label{eq:alphasq_cond}
    \dfrac{\hbar}{2 m_{A}\omega_A}=\left(\dfrac{2\alpha_{A}^{2}(0)}{9\pi}\right)^{\frac{1}{3}}\,\,.
\end{equation}
The three conditions in Eqs.\eqref{eq:alpha_cond},\eqref{eq:C6_CasPol} and \eqref{eq:alphasq_cond} allow to uniquely fix the parameters of each Drude oscillator representing the electronic response of each atom in terms of static polarizability and 
$C_{6}$-interaction coefficients, i.e.
\begin{equation}
\label{eq:QDO_parameters}
  \omega_{A}=\dfrac{4 C_{6AA}}{3\hbar\alpha_{A}^2(0)} \qquad m_{A}=\dfrac{3}{4}\left(\dfrac{9\pi}{16}\right)^{\frac{1}{3}}\dfrac{\hbar^2 \alpha_{A}^{\frac{4}{3}}(0)}{C_{6AA}} \qquad q_{A}=\left[\dfrac{4}{3}\left(\dfrac{9\pi}{16}\right)^{1/3}\dfrac{C_{6AA}}{\alpha^{\frac{5}{3}}_{A}}\right]^{\frac{1}{2}}\,\,.
\end{equation}
The values of the isotropic atomic polarizability $\alpha_{A}(0)$ and of the $C_{6AA}$ coefficients, to be substituted in the previous expressions for the QDOs parameters, have to take into account for the local environment of each atom in a molecule or in a larger complex.
For this reason the the DFT(B)+vdW(TS) scheme has been adopted: the static polarizabilities and the $C_{6}$ coefficient of  each atom in free space are rescaled with the ratio of the ratio of the atomic volumes in free space $V_{A,\text{free}}$ and in molecular environment  $V_{A,\text{DFT(B)}}$ both calculated using the Hirshfield "atom-in-molecule" partition scheme, i.e.
\begin{equation}
   \dfrac{C_{6AA,\text{TS}}}{C_{6AA,\text{free}}}=\left(\dfrac{\alpha_{\text{A,TS}}(0)}{\alpha_{\text{A,free}}(0)}\right)^2=\left(\dfrac{V_{A,\text{DFT(B)}}}{V_{A,\text{free}}}\right)^2\,\,\,.
\end{equation}

\section{Second quantization method applied to }

%  of the $A$-th atom in order to obtain the static atomic polarizability in molecular environment $\alpha_{A,\text{TS}}(0)$ assuming that the system has a finite electronic gap, i.e.

% where $V_{A,\text{free}}$,$V_{A}$ are respectively the atomic volume in
% in free space and in molecular environment calculated using the Hirshfield "atom-in-molecule" partition scheme.
